# Supplementary material for: XHand: Real-time Expressive Hand Avatar
Source: arXiv:2407.21002 source file (2024-07-30)
Supplement: Supplementary file 1 [file X_suppl.tex]

\section{More Details of Our Method}
\label{sec:more detail}

\subsection{MANO Subdivision}

The original MANO~\cite{MANO} mesh, consisting of 778 vertices and 1538 faces, has limited capacity to accurately represent fine-grained details~\cite{bib:handavatar}. To overcome this limitation by enhancing the mesh resolution to capture intricate features, we employ an uniform subdivision strategy on the MANO template mesh, as shown in Fig.~\ref{fig:mano}. By adding new vertices at midpoint of each edge, we obtain a refined mesh with 49,281 vertices and 98,432 faces. To associate skinning weights with these additional vertices, we compute the average weights assigned to the endpoints of the corresponding edges. Thus, we achieve a more comprehensive representation of hand morphology, which significantly improves the overall fidelity of the mesh.

\begin{figure}[htbp]
	\centering
        \vspace{-0.1in}
        \includegraphics[width=0.9\textwidth]{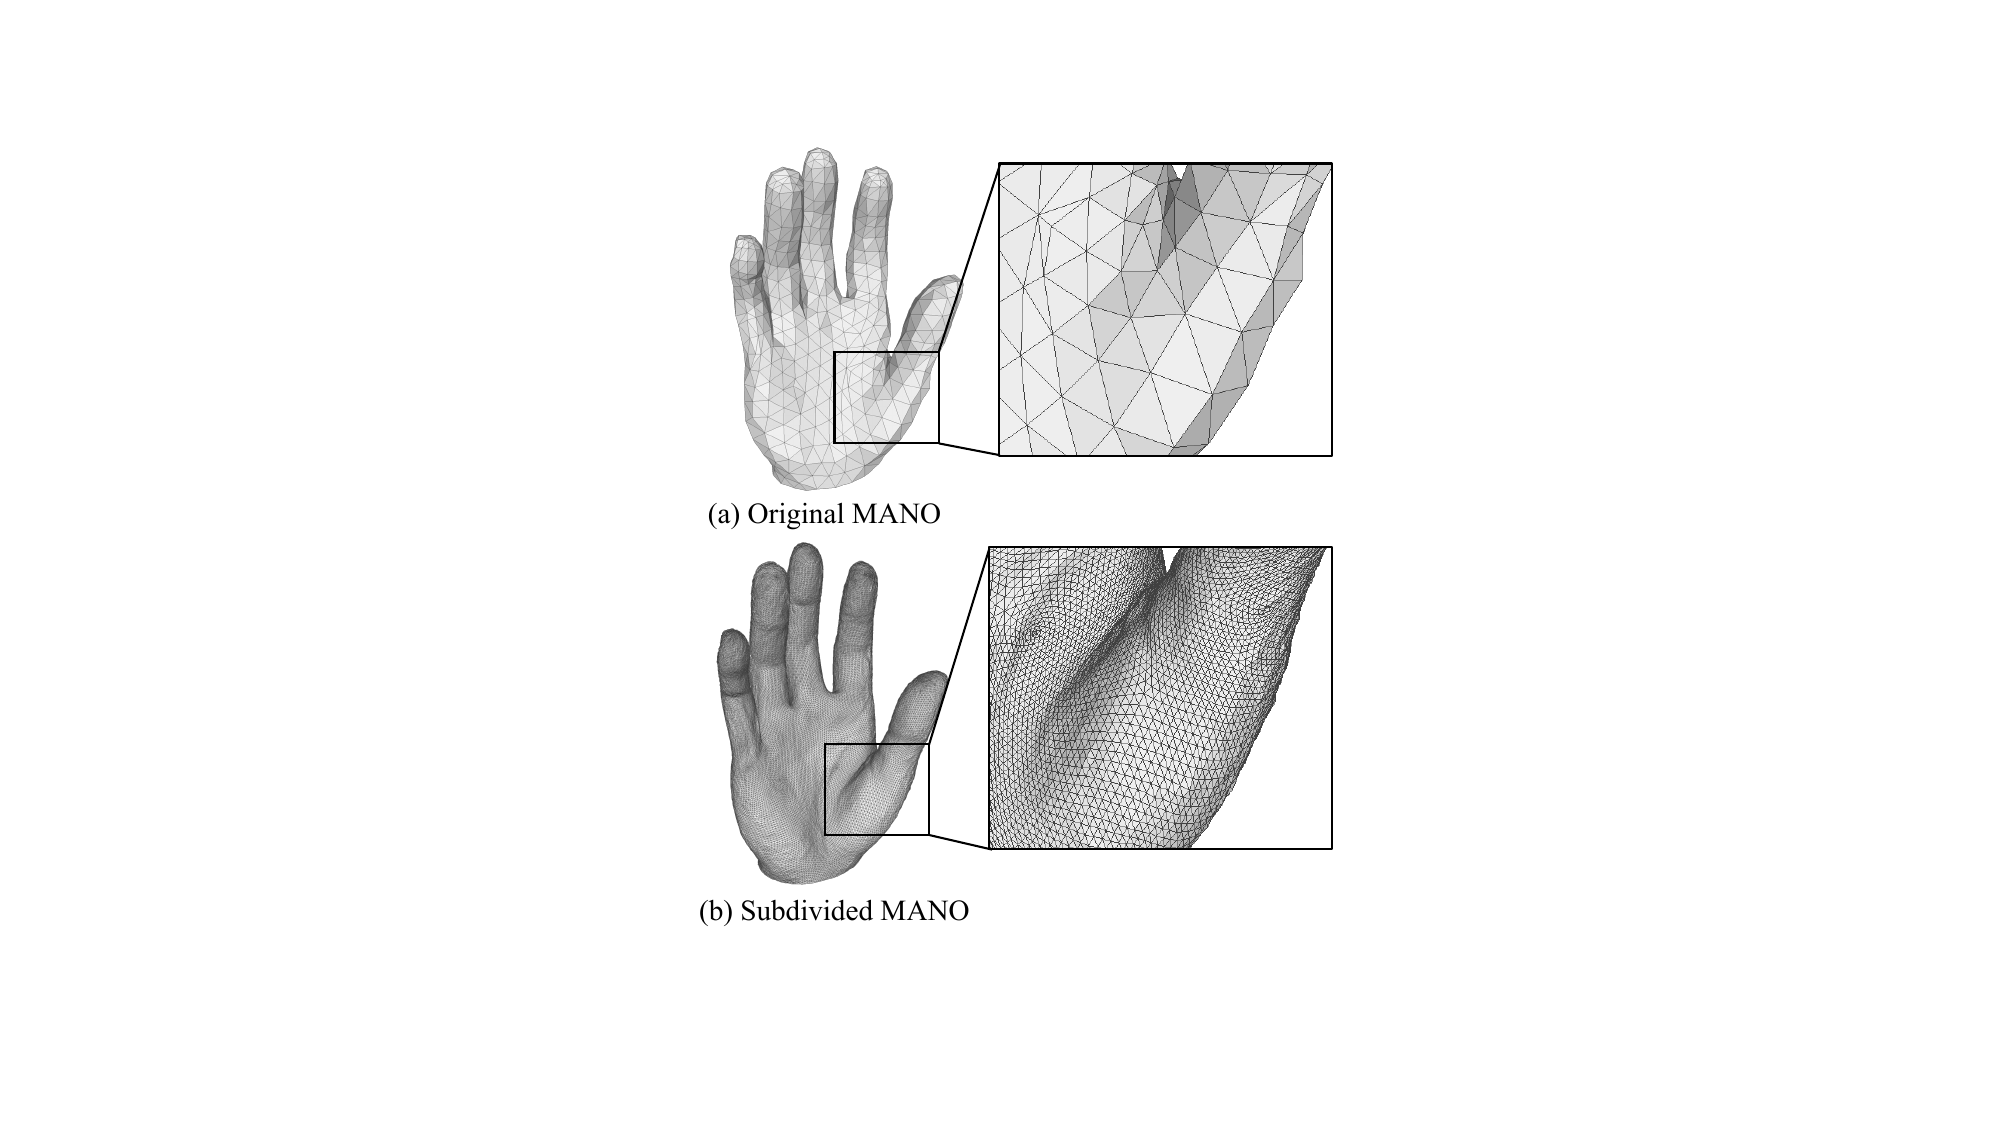}
        \vspace{-0.1in}
	\caption{The comparison of mesh refinement and texture between the original MANO and the subdivided MANO.}
	\label{fig:mano}
	\vspace{-0.2in}
\end{figure}

\subsection{Network Structures}

\begin{figure}[tb]
	\centering
	\begin{minipage}{0.45\linewidth}
        \vspace{-0.1in}
        \centering
        \includegraphics[width=0.7\textwidth]{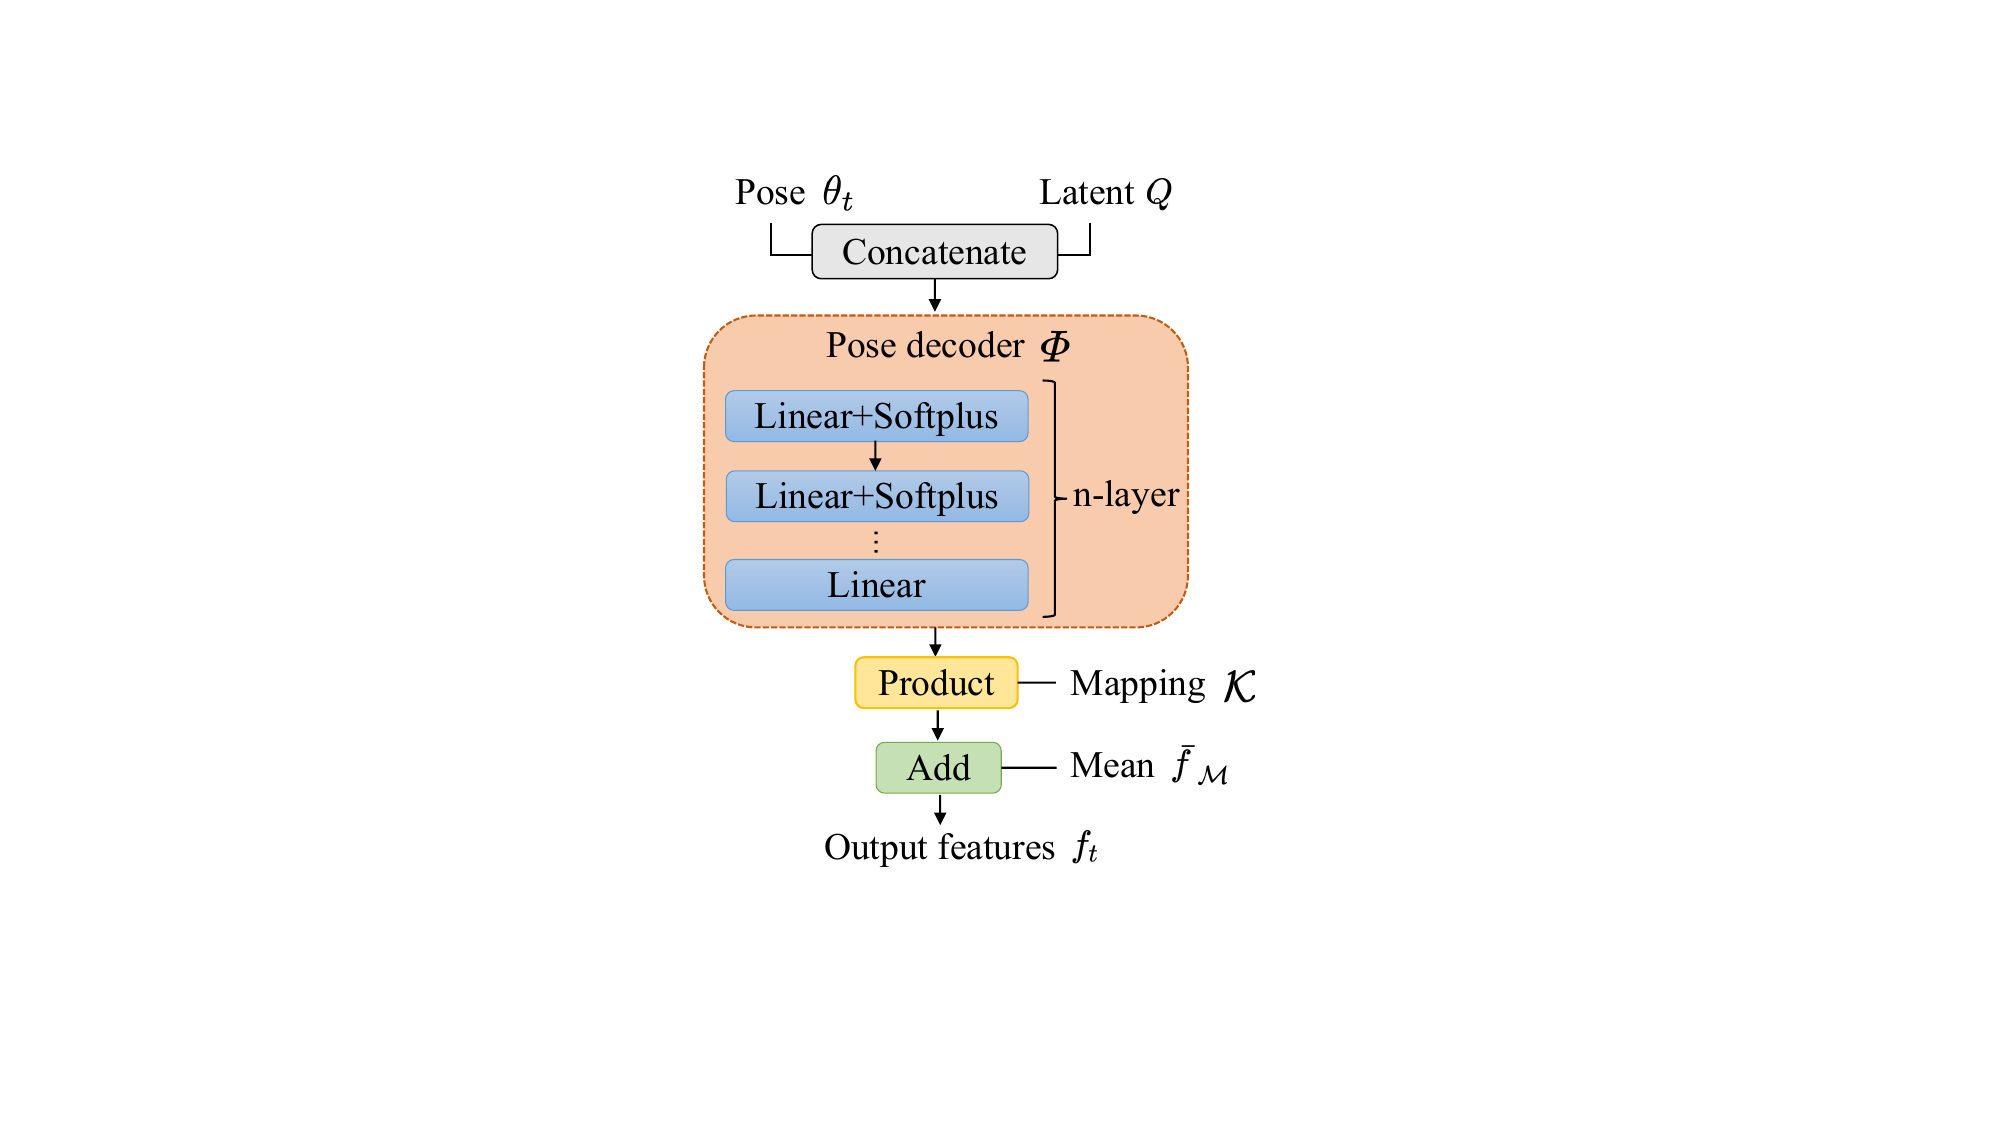}
        \vspace{-0.1in}
    	\caption{The structure of feature embedding module $\Psi$, where pose decoder consists linear layers with Softplus activations.}
    	\label{fig:fe}
    	\vspace{-0.2in}
	\end{minipage}
		\begin{minipage}{0.45\linewidth}
        \vspace{-0.1in}
        \centering
        \includegraphics[width=0.45\textwidth]{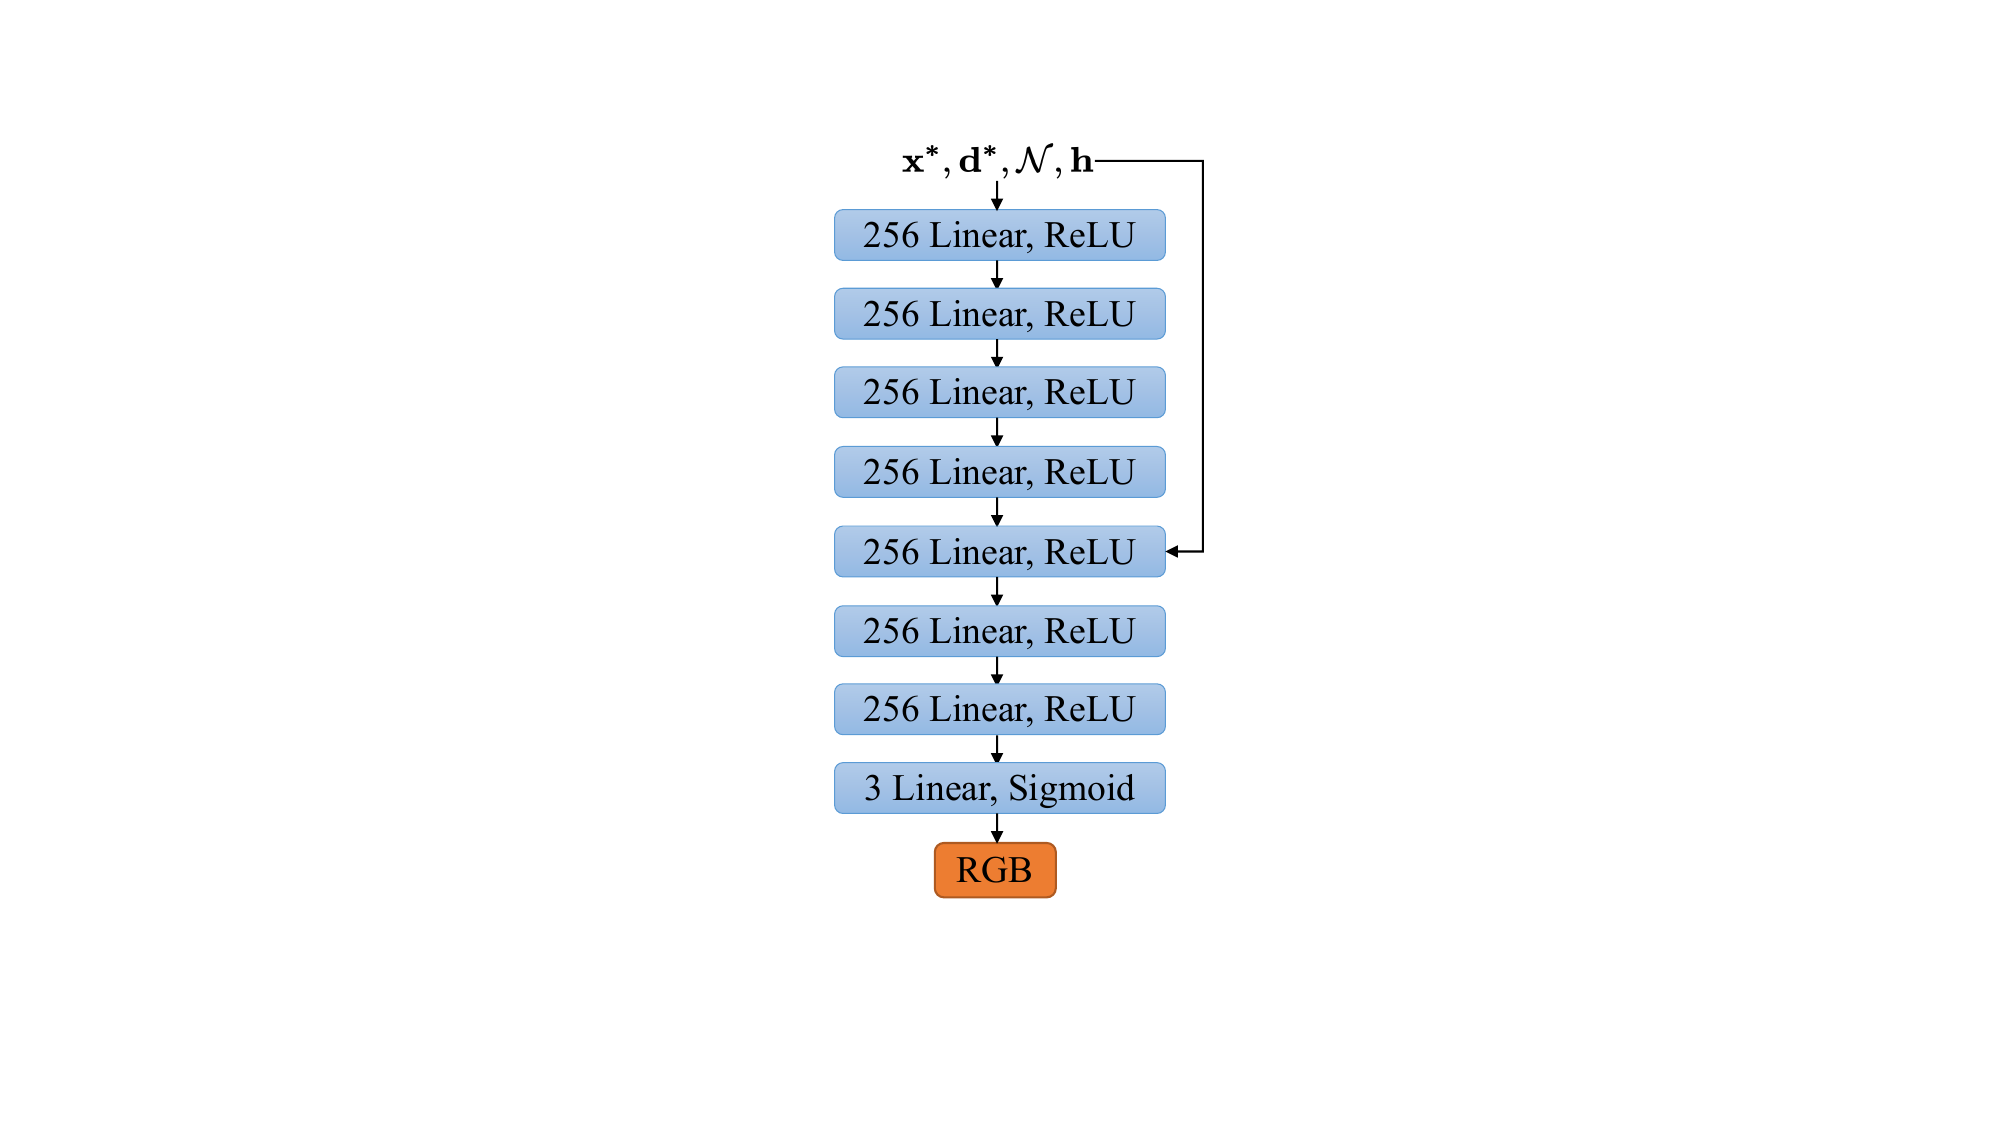}
        \vspace{-0.1in}
    	\caption{The structure of neural renderer $\mathcal{C}$, where $*$ donates positional encoding~\cite{aliev2020neural} operation.}
    	\label{fig:nr}
    	\vspace{-0.2in}
	\end{minipage}
\end{figure}

\noindent\textbf{Pose Decoder.} For decode the pose $\theta_t$ at time $t$ and the vertex latent code $Q$, pose decoder $\Phi$ in the feature embedding module is designed with a multi-layer MLP with Softplus activation functions. The depths of $\Phi_{lbs}$ in LBS embedding module $\Psi_{lbs}$ and $\Phi_{D}$ in displacement embedding module $\Psi_D$ are set to 5, where the number of neurons is 128. The depth of $\Phi_{\rho}$ in albedo embedding module $\Psi_{\rho}$ is 8, where the number of neurons is 512.

\noindent\textbf{Neural Network.} Based on Mildenhall~\textit{et al.}~\cite{NeRF}, the neural network $\mathcal{C}$ consists of 8 fully-connected layers with ReLU activations and 256 channels per layer. Additionally, it incorporates a skip connection that concatenates the input to the activation of the fifth layer.

The structure of pose decoder $\Phi$ 
 in feature embedding module $\Psi$ can be found in Fig.~\ref{fig:fe} and the constructional details of neural network $\mathcal{C}$ are shown in Fig.~\ref{fig:nr}.

% \subsection{Training Details}

% \noindent\textbf{Back-propagation.} In the training process of XHand, it is important to note that the backpropagation of various loss functions involves with different objectives. Specifically, $\mathcal{L}_{inv}$ is backpropagated to three feature embeddings: $\Psi_{D}$, $\Psi_{lbs}$ and $\Psi_{\rho}$, aiming to learn the generation of fine meshes. While, in the training process of the neural renderer $\mathcal{C}$, the latent codes $Q_D$ and $Q_\rho$ obtained from the feature embeddings are treated as the detached. Therefore, $L_{neu}$ is only used to learn the neural renderer $\mathcal{C}$ and render latent codes $Q_{render}$.

\section{Additional Results}

\subsection{Choices of Neural Rendering}
Traditional neural radiance fields~\cite{NeRF} utilize an 8-layer MLP as the renderer. In contrast, our mesh-based network eliminates the need for point cloud sampling and enables direct rendering through vertex features. Consequently, our neural renderer makes use of UNet~\cite{unet} that takes advantage of topology consistency. This allows our method to achieve promising performance. To investigate this, we performed ablation experiments on both network architectures, as presented in Table~\ref{tab:mlp-unet}. The experiments demonstrate that UNet with 4 layers yields the superior rendering quality, albeit at the cost of inference speed. On the other hand, MLPs can enhance performance by 20\% with only a marginal loss in accuracy. Therefore, MLPs are employed as our neural renderer. Furthermore, our investigation into a well-designed image generation network, EG3D~\cite{chan2022efficient}, reveals its unsuitability for neural rendering.

\begin{table}[htbp]
    \centering
    \caption{Rendering quality and inference speed comparisons between EG3D~\cite{chan2022efficient}, UNet and MLPs used in neural rendering.}
	\begin{tabular}{c | c c c c}
            \toprule
            \textbf{Method} & LPIPS $\downarrow$ & PSNR $\uparrow$ & SSIM $\uparrow$ & FPS $\uparrow$\\
            \hline 
            XHand-MLPs  & 0.012  & 34.32  & 0.986 & \bf56.2 \\
            XHand-UNet  & \bf0.011  & \bf34.72  & \bf0.987 & 46.2 \\
            XHand-EG3D~\cite{chan2022efficient}  & 0.013  & 32.3  & 0.981 & 40.4 \\
            \bottomrule
	\end{tabular}
  \vspace{-0.05in}
 \label{tab:mlp-unet}
\end{table}

% \noindent\textbf{Length of Latent Code.}

\subsection{Novel Pose Synthesis}

\begin{figure*}
    \vspace{-0.2in}
	\centering
        \includegraphics[width=0.65 \linewidth]{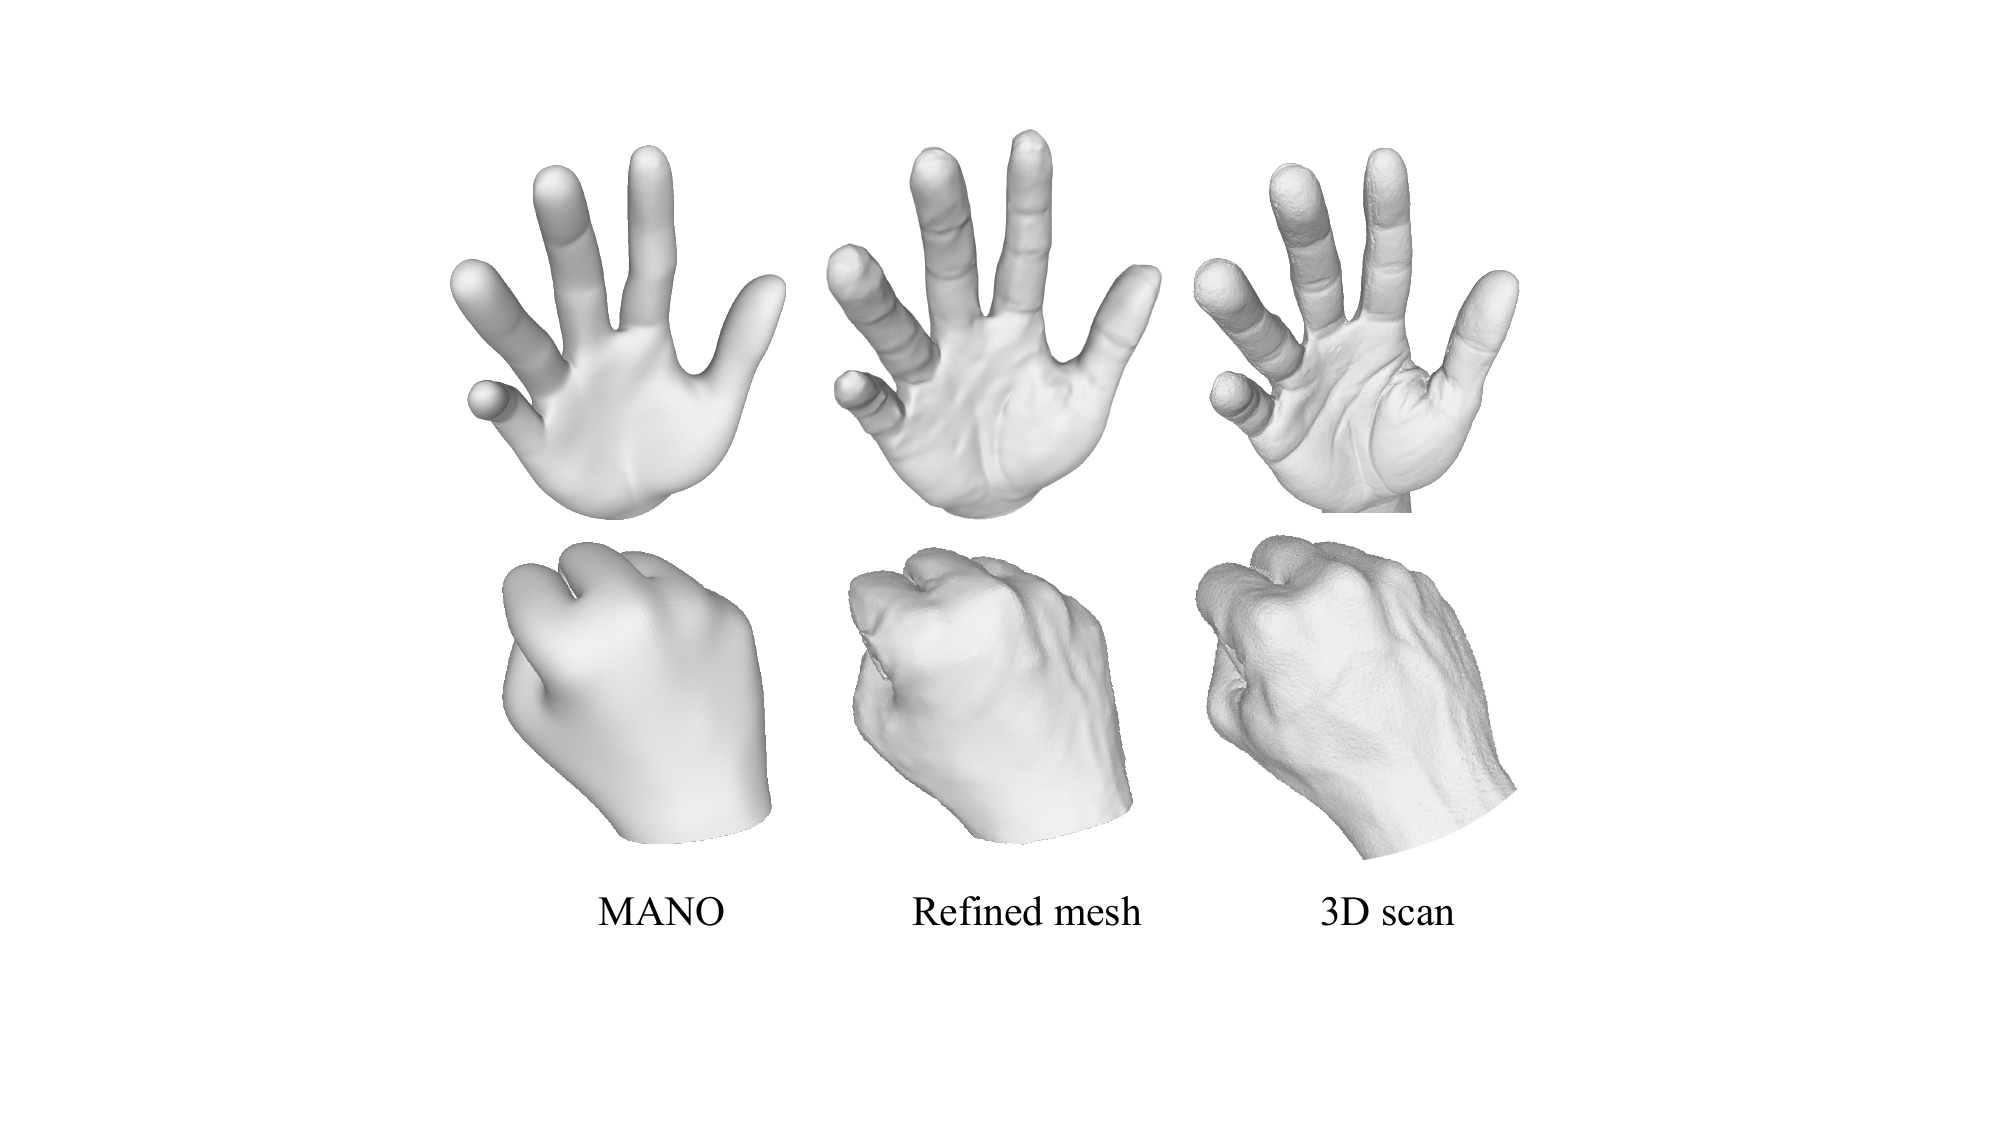}
        % \vspace{-0.1in}
	\caption{More visual results on DeepHandMesh~\cite{Moon_2020_ECCV_DeepHandMesh}.}
	\label{fig:dhm}
	\vspace{-0.2in}
\end{figure*}

In addition to the visual results presented in the main paper, more experimental results conduct on DeepHandMesh~\cite{Moon_2020_ECCV_DeepHandMesh} dataset are visualized in Fig.~\ref{fig:dhm}. Moreover, we provide a video named ``\texttt{demo.mp4}'' to better demonstrate the effectiveness of our proposed approach on novel pose synthesis. We show the XHand avatars obtained from InterHand2.6M~\cite{Moon_2020_ECCV_InterHand2.6M} dataset with different pose sequences. The video contains the comparison results with real images from InterHand2.6M, demonstrations driven by new poses, and a display driven by wild videos for XHand avatar. More results are illustrated in Fig.~\ref{fig:moreresults} and Fig.~\ref{fig:wild}. %The video provides a comprehensive demonstration of the performance and potential of our method.
%We further provide a video demo named ``\texttt{demo.mp4}'' to demonstrate the capability of our method. In the video, we present visualizations of the temporal sequences, including results on InterHand2.6M and a new pose sequences.

\begin{figure*}[htp]
	\centering
        \includegraphics[width=0.93 \linewidth]{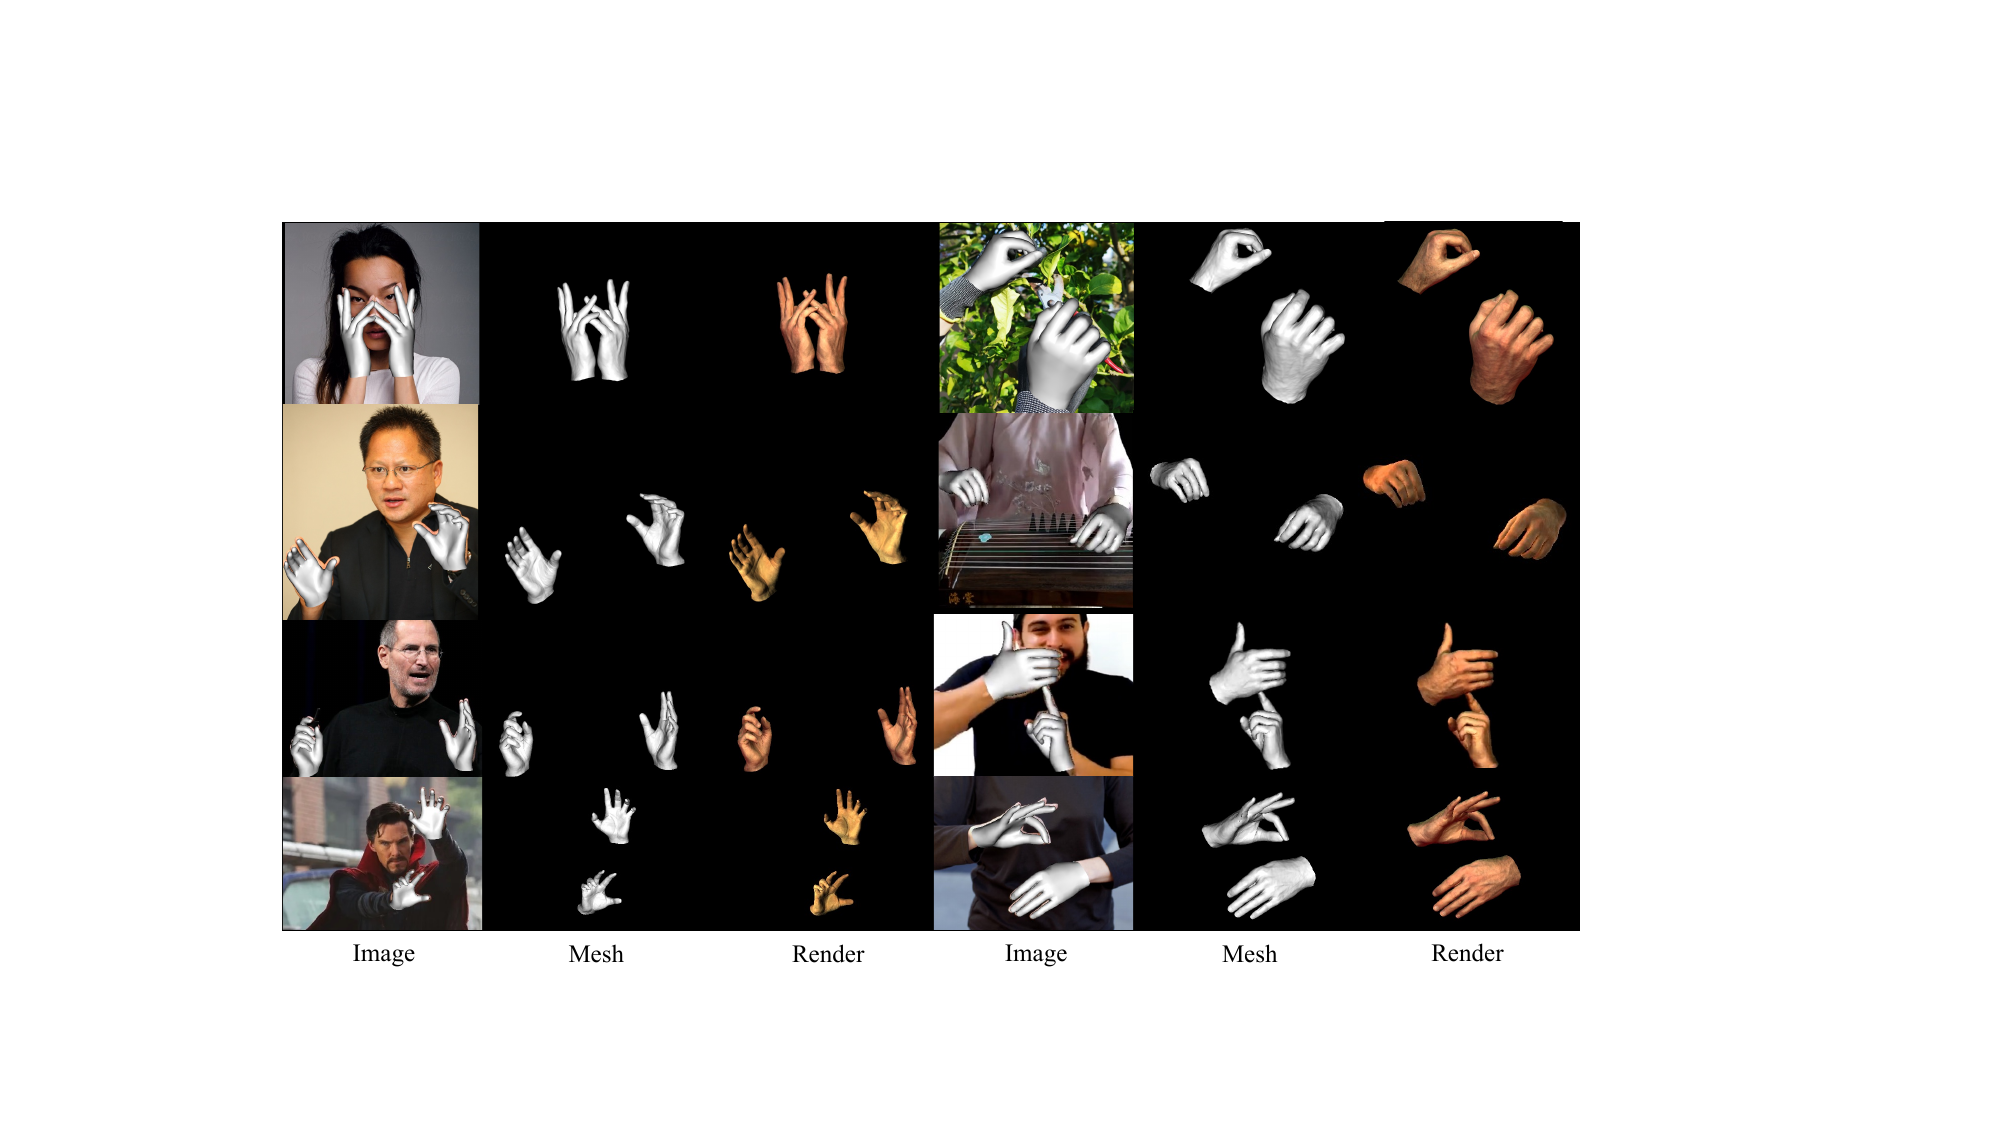}
        \vspace{-0.1in}
	\caption{More visual results on wild images. The MANO parameters are extracted from Hamer~\cite{pavlakos2023reconstructing}.}
	\label{fig:wild}
	\vspace{-0.2in}
\end{figure*}

\begin{figure*}[h]
	\centering
        \includegraphics[width=0.7 \linewidth]{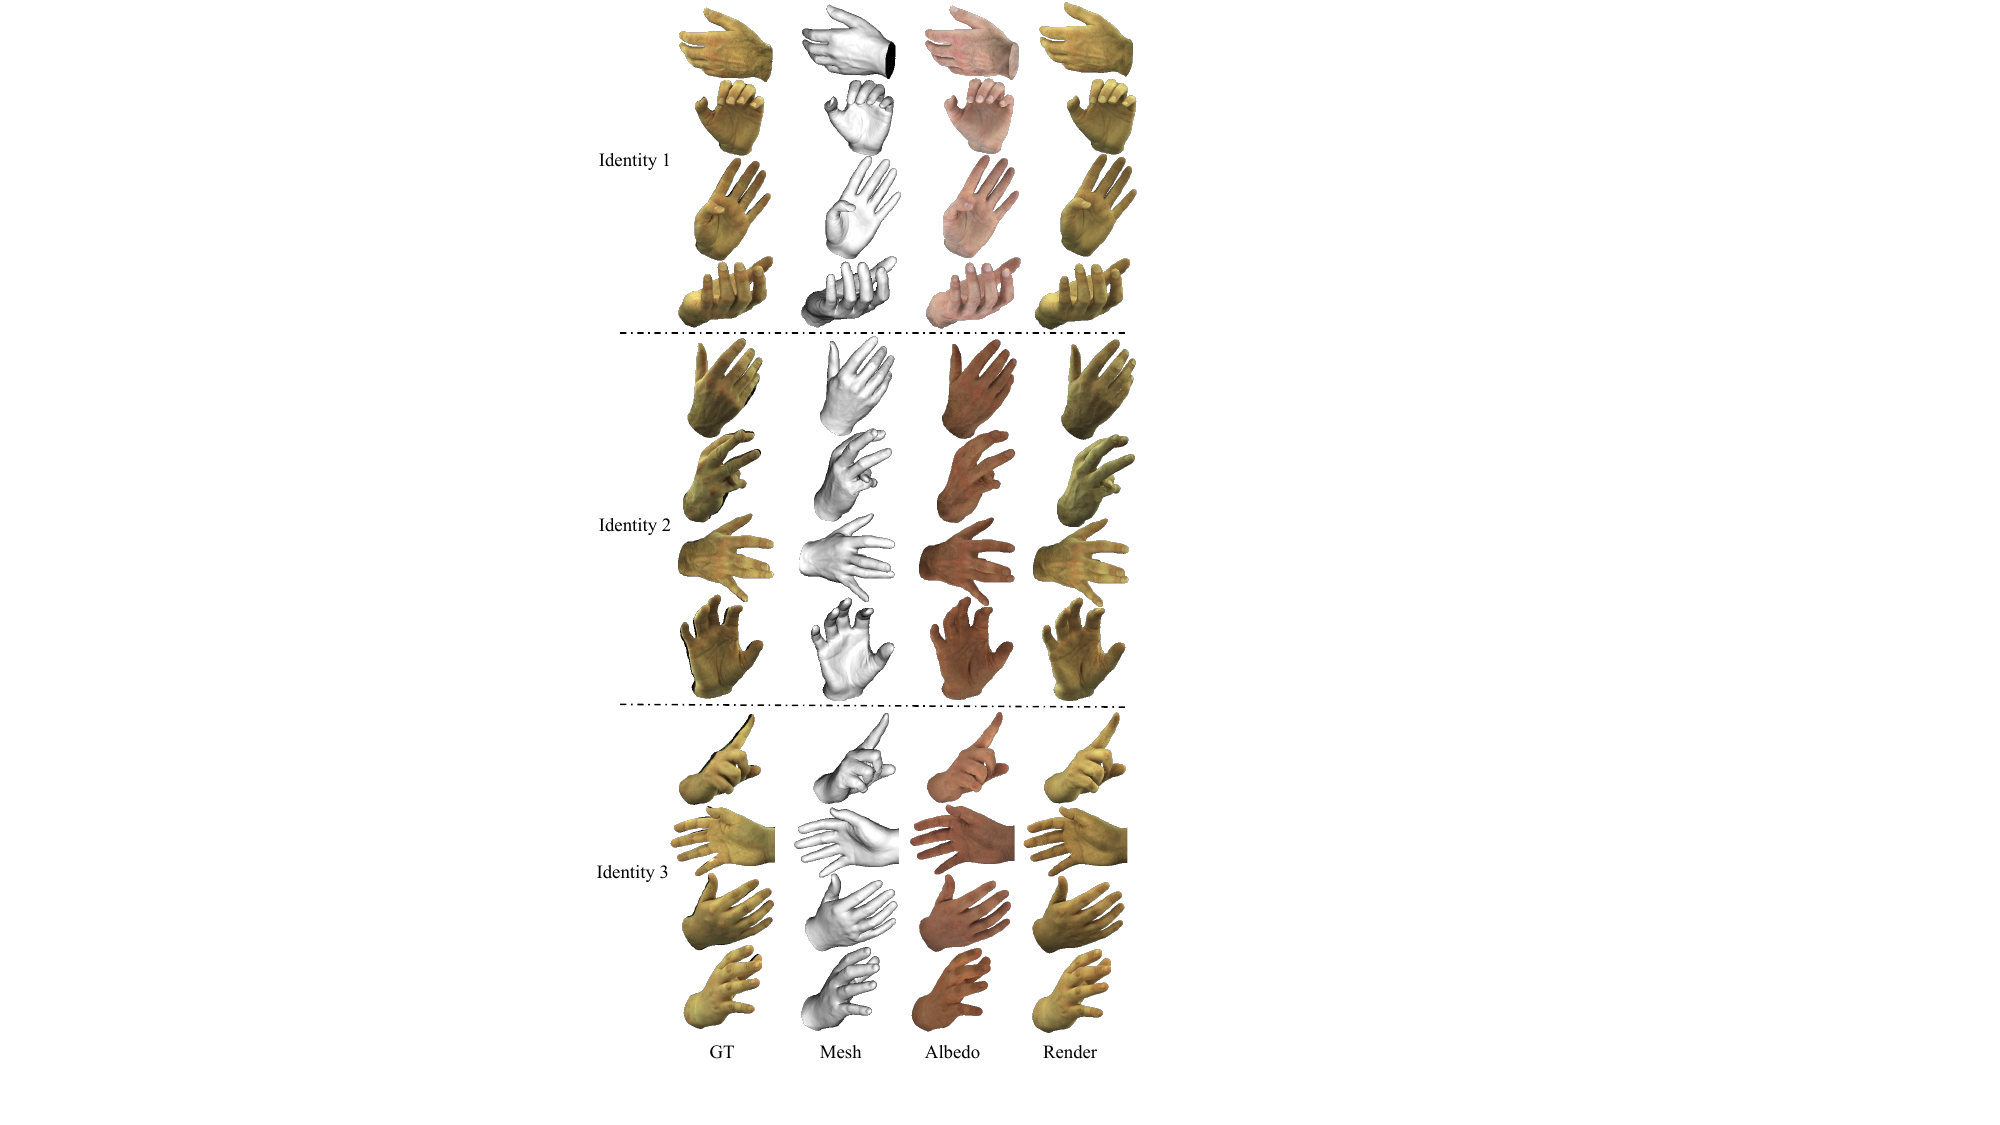}
        \vspace{-0.1in}
	\caption{More visual results on InterHand2.6M~\cite{Moon_2020_ECCV_InterHand2.6M}.}
	\label{fig:moreresults}
	\vspace{-0.2in}
\end{figure*}
